# Supplementary material for: BiSPARCs for Unsourced Random Access in Massive MIMO
Source: arXiv:2304.14546 source file (2023-04-27)
Supplement: Supplementary file 1 [file 07_appendix_old.tex]

\input{tables/message_approximations.tex}
\section{Derivation of Message Approximations}\label{sec:message-derivation}
Message computations require high-dimensional integration and normalization. To reduce the computational complexity, we approximate these messages by following the general idea of the \ac{AMP} framework \cite{parker_bilinear_2014,Donoho,Rangan11}. To facilitate the approximations, we define the mean and variance quantities in Table~\ref{tbl:updates}. Specifically, we derive the message in the large-system limit, i.e, $N,K,M,T\rightarrow \infty$ with fixed ratios for $M/N$, $K/N$ and $T/N$. Without loss of generality, we assume that $h_{km}$ scales with $O(1/\sqrt{M})$ and $A_{tn}$ scales with $O(1/\sqrt{T})$, other quantities scale as $O(1)$.

Under the large-system limit, i.e., $N,K,L,T\rightarrow \infty$ with fixed ratios, we can approximate $p^i(w_{nm})$ by a Gaussian distribution, with mean $\hat{p}_{nm}(i)$ and variance $v^p_{nm}(i)$ given by 
\begin{align}
    \hat{p}_{nm}(i) = &\sum\limits_{k=1}^{K}\hat{c}_{nk}\hat{h}_{km}\\
    \begin{split}
        v^p_{nm}(i)={}& \sum\limits_{k=1}^{K}\vert\hat{c}_{nk}\vert^2v^h_{km,n}(i)+v^c_{nk,m}(i)\vert\hat{h}_{km,n}\vert^2\\
        &+v^c_{nk,m}(i)v^h_{km,n}(i)    
    \end{split}
\end{align}
Then, we employ the methodology in the derivation of AMP \cite{parker_bilinear_2014} to approximate \eqref{eq:first_message}-\eqref{eq:first_update}. Based on the central limit theorem argument, we approximate $\prod_{l\neq n}\Delta_{f_{lm}\rightarrow z_{tm}}^{i}$ in \eqref{eq:first_message} by a Gaussian distribution, i.e., $\M{f_{nm}}{z_{tm}}{(i)}{w_{nm}}\approx \CN{w_{nm}}{\hat{w}_{nm,t}(i)}{v^{w}_{nm,t}(i)}$. The mean and variance are given by 
\begin{align}
    \hat{w}_{nm,t}(i+1)&=\hat{w}_{nm}(i+1)-v^{w}_{nm}(i+1)A_{tn}\hat{\tau}_{t,m}(i)\\
    v^{w}_{nm,t}(i+1)&=v^{w}_{nm}(i+1)
\end{align}
with 
\begin{align}
    v^{w}_{nm}(i+1)&=\frac{v^{p}_{nm}(i)v^{\zeta}_{nm}(i)}{v^{p}_{nm}(i)+v^{\zeta}_{nm}(i)},\\
    \hat{w}_{nm}(i+1)&=v^{w}_{nm}(i+1)\left(\frac{\hat{\zeta}_{nm}(i)}{v^{\zeta}_{nm}(i)}+\frac{\hat{p}_{nm}(i)}{v^{p}_{nm}(i)}\right)
\end{align}
where the auxiliary variables are given by 
\begin{subequations}
    \label{eq:auxiliary}
    \begin{align}
        v^u_{tm}(i)&=\sum\limits_{t=1}^T\vert A_{tn}\vert^2 v^w_{tm}(i),\\
        \hat{u}_{tm}(i)&=\sum\limits_{n=1}^N A_{tn}\hat{w}_{nm}(i)-v_{tm}^u(i)\hat{\tau}_{tm}(i-1),\label{eq:onsager}\\
        v^z_{tm}(i)&=\frac{v^u_{tm}(i)\sigma^2}{v^u_{tm}(i)+\sigma^2},\\
        \hat{z}_{tm}(i)&=\frac{\hat{u}_{tm}(i)\sigma^2+y_{tm}v_{tm}^u(i)}{v_{tm}^u(i)+\sigma^2},\\
        v^{\tau}_{tm}(i)&=\frac{\hat{u}_{tm}(i)-v_{tm}^z(i)}{\vert v_{tm}^u(i)\vert^2},\\
        \hat{\tau}_{tm}(i)&=\frac{\hat{z}_{tm}(i)-\hat{u}_{tm}(i)}{v^u_{tm}(i)},\\
        v_{nm}^{\zeta}(i)&=\left(\sum\limits_{t=1}^T \vert A_{tn}\vert^2 v^{\tau}_{tm}(i)\right)^{-1},\label{eq:w1}\\
        \hat{\zeta}_{nm}(i)&=\hat{w}_{nm}(i)+v_{nm}^{\zeta}(i)\sum\limits_{t=1}^TA_{tn}^{*}\hat{\tau}_{tm}(i).\label{eq:w2}
    \end{align}
\end{subequations}
Note that in \eqref{eq:onsager}, a first-order correction term is introduced, which is similar to the Onsager correction term of AMP, e.g. \cite{parker_bilinear_2014}. By \eqref{eq:w1} and \eqref{eq:w2} we have 
\begin{equation}
    \prod_{t=1}^T\M{z_{tm}}{f_{nm}^w}{(i)}{w_{nm}}\approx \mathcal{CN}(w_{nm};\hat{\zeta}_{nm}(i),v_{nm}^{\zeta}(i)).\label{eq:pdf_ztilde}
\end{equation}
Substituting \eqref{eq:pdf_ztilde} into \eqref{eq:second_message} and \eqref{eq:third_message}, we find that the form of \eqref{eq:second_message} matches that in eq (13) of \cite{parker_bilinear_2014}. Following Sction II.D-F in \cite{parker_bilinear_2014}, we compute $\hat{p}_{nm}(i)$ and $v_{nm}^p(i)$ and close the loop as
\begin{subequations}
    \label{eq:auxiliary2}
    \allowdisplaybreaks
    \begin{align}
        \begin{split}
            v_{nm}^p(i)={}&\sum_k\vert\hat{c}_{nk}(i)\vert^2v_{km}^h(i)\\
            &+v_{nk}^c(i)\vert \hat{h}_{km}(i)\vert^2+v_{nk}^c(i)v_{km}^h(i),
        \end{split}\\
        \begin{split}
            \hat{p}_{nm}(i)={}&\sum_k \hat{c}_{nk}(i)\hat{h}_{km}(i)-\hat{\alpha}_{nk}(i-1)\\
            &\sum_k(\vert\hat{c}_{nk}(i)\vert^2 v_{km}^h(i)+v_{nk}^c(i)\vert\hat{h}_{km}(i)\vert^2),
        \end{split}\\
        v_{nm}^{\alpha}(i)={}&(v_{nm}^p(i)+v_{nm}^{\zeta}(i))^{-1},\\
        \hat{\alpha}_{nm}(i)={}&\frac{\hat{\zeta}_{nk}(i)-\hat{p}_{nk}(i)}{v^p_{nk}(i)+v^{\zeta}_{nk}(i)},\\
        \begin{split}
            v_{km}^r(i)={}&(\sum_n \vert\hat{c}_{nk}(i)\vert^2v_{nk}^{\alpha}(i))^{-1},
        \end{split}\\
        \begin{split}
            \hat{r}_{km}(i)={}&\hat{h}_{km}(i)(1-v^r_{km}(i)\sum_n v_{nk}^c(i)v_{nk}^{\alpha}(i))\\
            &+v^r_{km}(i)\sum_n\hat{c}^*_{nk}(i)\hat{\alpha}_{nk}(i),
        \end{split}\\
        v^q_{nk}(i)={}&(\sum_m\vert\hat{h}_{km}(i)\vert^2v_{nm}^{\alpha}(i))^{-1},\\
        \begin{split}
            \hat{q}_{nk}(i)={}&\hat{c}_{nk}(i)(1-v_{nk}^q(i)\sum_m v_{km}^h(i)v_{nm}^{\alpha}(i))\\
            &+v_{nk}^q(i)\sum_m\hat{h}^*_{km}(i)\hat{\alpha}_{nk}(i),
        \end{split}
    \end{align}
\end{subequations}
where 
\begin{subequations}
    \label{eq:auxiliary}
    \begin{align}
        \hat{h}_{km}(i+1)&=\int_{h_{km}}h_{km}\Delta_{h_{km}}^i(h_{km})\label{eq:channel1},\\
        v_{km}^{h}(i+1)&=\int_{h_{km}}h_{km}^2\Delta_{h_{km}}^i(h_{km})-\vert\hat{h}_{km}(i+1)\vert^2\label{eq:channel2},\\
        \hat{c}_{nk}(i+1)&=\int_{c_{nk}}c_{nk}\Delta_{c_{nk}}^i(c_{nk})\label{eq:bcode1},\\
        v_{nk}^{c}(i+1)&=\int_{c_{nk}}c_{nk}^2\Delta_{c_{nk}}^i(c_{nk})-\vert\hat{c}_{nk}(i+1)\vert^2\label{eq:bcode2}
    \end{align}
\end{subequations}
The resulting messages and posteriors after the approximations are shown in Table~\ref{tbl:updates}, where $Z$ denotes a normalization factor that ensures the messages are integrated to $1$.

% Under the large-system limit, i.e., $N,K,L,T\rightarrow \infty$ with fixed ratios, we can approximate $P_{w_{nm}}^i(w_{nm})$ by a Gaussian distribution, with mean $\hat{p}_{nm}(i)$ and variance $v^p_{nm}(i)$ given by 
% \begin{align}
%     \hat{p}_{nm}(i) = &\sum\limits_{k=1}^{K}\hat{s}_{nk}\hat{h}_{km}\\
%     v^p_{nm}(i)={}& \sum\limits_{k=1}^{K}\vert\hat{s}_{nk}\vert^2v^h_{km,n}(i)+v^s_{nk,m}(i)\vert\hat{h}_{km,n}\vert^2+v^s_{nk,m}(i)v^h_{km,n}(i)    
% \end{align}
% Then, we employ the methodology in the derivation of AMP \cite{parker_bilinear_2014} to approximate \eqref{eq:first_message}-\eqref{eq:first_update}. Based on the central limit theorem argument, we approximate $\prod_{l\neq n}\Delta_{f_{lm}\rightarrow z_{tm}}^{i}$ in \eqref{eq:first_message} by a Gaussian distribution, i.e., $\M{f_{nm}}{z_{tm}}{i}{w_{nm}}\approx \mathcal{CN}(w_{nm};\hat{w}_{nm,t}(i),v^{w}_{nm,t}(i))$. The mean and variance are given by 
% \begin{align}
%     \hat{w}_{nm,t}(i+1)&=\hat{w}_{nm}(i+1)-v^{w}_{nm}(i+1)C_{tn}\hat{\tau}_{t,m}(i)\\
%     v^{w}_{nm,t}(i+1)&=v^{w}_{nm}(i+1)
% \end{align}
% with 
% \begin{align}
%     v^{w}_{nm}(i+1)&=\frac{v^{p}_{nm}(i)v^{\zeta}_{nm}(i)}{v^{p}_{nm}(i)+v^{\zeta}_{nm}(i)},\\
%     \hat{w}_{nm}(i+1)&=v^{w}_{nm}(i+1)\left(\frac{\hat{\zeta}_{nm}(i)}{v^{\zeta}_{nm}(i)}+\frac{\hat{p}_{nm}(i)}{v^{p}_{nm}(i)}\right)
% \end{align}
% where the auxiliary variables are given by 
% \begin{subequations}
%     \label{eq:auxiliary}
%     \begin{align}
%         v^u_{tm}(i)&=\sum\limits_{t=1}^T\vert C_{tn}\vert^2 v^w_{tm}(i),\\
%         \hat{u}_{tm}(i)&=\sum\limits_{n=1}^N C_{tn}\hat{w}_{nm}(i)-v_{tm}^u(i)\hat{\tau}_{tm}(i-1),\label{eq:onsager}\\
%         v^z_{tm}(i)&=\frac{v^u_{tm}(i)\sigma^2}{v^u_{tm}(i)+\sigma^2},\\
%         \hat{z}_{tm}(i)&=\frac{\hat{u}_{tm}(i)\sigma^2+y_{tm}v_{tm}^u(i)}{v_{tm}^u(i)+\sigma^2},\\
%         v^{\tau}_{tm}(i)&=\frac{\hat{u}_{tm}(i)-v_{tm}^z(i)}{\vert v_{tm}^u(i)\vert^2},\\
%         \hat{\tau}_{tm}(i)&=\frac{\hat{z}_{tm}(i)-\hat{u}_{tm}(i)}{v^u_{tm}(i)},\\
%         v_{nm}^{\zeta}(i)&=(\sum\limits_{t=1}^T \vert C_{tn}\vert^2 v^{\tau}_{tm}(i))^{-1},\label{eq:w1}\\
%         \hat{\zeta}_{nm}(i)&=\hat{w}_{nm}(i)+v_{nm}^{\zeta}(i)\sum\limits_{t=1}^TC_{tn}^{*}\hat{\tau}_{tm}(i).\label{eq:w2}
%     \end{align}
% \end{subequations}
% Note that in \eqref{eq:onsager}, a first-order correction term is introduced, which is similar to the Onsager correction term of AMP, e.g. \cite{parker_bilinear_2014}. By \eqref{eq:w1} and \eqref{eq:w2} we have 
% \begin{equation}
% \prod_{t=1}^T\M{z_{tm}}{f_{nm}^w}{i}{w_{nm}}\approx \mathcal{CN}(w_{nm};\hat{\zeta}_{nm}(i),v_{nm}^{\zeta}(i)).\label{eq:pdf_ztilde}
% \end{equation}
% Substituting \eqref{eq:pdf_ztilde} into \eqref{eq:second_message} and \eqref{eq:third_message}, we find that the form of \eqref{eq:second_message} matches that in eq (13) of \cite{parker_bilinear_2014}. Following Sction II.D-F in \cite{parker_bilinear_2014}, we compute $\hat{p}_{nm}(i)$ and $v_{nm}^p(i)$ and close the loop as
% \begin{subequations}
% \label{eq:auxiliary2}
% \begin{align}
% v_{nm}^p(i)=&\sum_k\vert\hat{s}_{nk}(i)\vert^2v_{km}^h(i)+v_{nk}^s(i)\vert \hat{h}_{km}(i)\vert^2+v_{nk}^s(i)v_{km}^h(i),\\
% \hat{p}_{nm}(i)=&\sum_k \hat{s}_{nk}(i)\hat{h}_{km}(i)-\hat{\alpha}_{nk}(i-1)\sum_k(\vert\hat{s}_{nk}(i)\vert^2 v_{km}^h(i)+v_{nk}^s(i)\vert\hat{h}_{km}(i)\vert^2),\\
% v_{nm}^{\alpha}(i)=&(v_{nm}^p(i)+v_{nm}^{\zeta}(i))^{-1},\\
% \hat{\alpha}_{nm}(i)=&\frac{\hat{\zeta}_{nk}(i)-\hat{p}_{nk}(i)}{v^p_{nk}(i)+v^{\zeta}_{nk}(i)},\\
% v_{km}^r(i)=&(\sum_n \vert\hat{s}_{nk}(i)\vert^2v_{nk}^{\alpha}(i))^{-1},\\
% \hat{r}_{km}(i)=&\hat{h}_{km}(i)(1-v^r_{km}(i)\sum_n v_{nk}^s(i)v_{nk}^{\alpha}(i))+v^r_{km}(i)\sum_n\hat{s}^*_{nk}(i)\hat{\alpha}_{nk}(i),\\
% v^q_{nk}(i)=&(\sum_m\vert\hat{h}_{km}(i)\vert^2v_{nm}^{\alpha}(i))^{-1},\\
% \hat{q}_{nk}(i)=&\hat{s}_{nk}(i)(1-v_{nk}^q(i)\sum_m v_{km}^h(i)v_{nm}^{\alpha}(i))+v_{nk}^q(i)\sum_m\hat{h}^*_{km}(i)\hat{\alpha}_{nk}(i),
% \end{align}
% \end{subequations}
% where 
% \begin{subequations}
%     \label{eq:auxiliary}
%     \begin{align}
%         \hat{h}_{km}(i+1)&=\int_{h_{km}}h_{km}\Delta_{h_{km}}^i(h_{km}),\\
%         v_{km}^{h}(i+1)&=\int_{h_{km}}h_{km}^2\Delta_{h_{km}}^i(h_{km})-\vert\hat{h}_{km}(i+1)\vert^2,\\
%         \hat{s}_{nk}(i+1)&=\int_{s_{nk}}s_{nk}\Delta_{s_{nk}}^i(s_{nk}),\\
%         v_{nk}^{s}(i+1)&=\int_{s_{nk}}s_{nk}^2\Delta_{s_{nk}}^i(s_{nk})-\vert\hat{s}_{nk}(i+1)\vert^2
%     \end{align}
% \end{subequations}
% The resulting messages and posteriors after the approximations are shown in Table~\ref{tbl:updates}, where $Z$ denotes a normalization factor that ensures the messages are integrated to $1$.

\section{Calculation of Posterior Update Messages}

Given the Rayleigh fading assumption, \eqref{eq:channel1} and \eqref{eq:channel2} are be readily given by
\begin{subequations}
    \begin{align}
        \hat{h}_{km}(i+1)&=\frac{\hat{r}_{km}(i)}{1+v_{km}^r(i)}\label{eq:channel_update},\\
        v_{km}^{h}(i+1)&=\frac{v^r_{km}(i)}{1+v_{km}^r(i)}\label{eq:channel_var_update},
    \end{align}
\end{subequations}
and for the binary codewords in \eqref{eq:bcode1} and \eqref{eq:bcode2}, we get
\begin{subequations}
    \begin{align}
         \hat{c}_{nk}(i+1)&=\frac{1}{1+\frac{(1-\epsilon_{nk})}{\epsilon_{nk}}\exp(\frac{1-2\mathrm{Re}\{\hat{q}_{nk}(i)\}}{v^{q}_{nk}(i)})}\label{eq:code_update},\\
        v_{nk}^{c}(i+1)&=\frac{\frac{(1-\epsilon_{nk})}{\epsilon_{nk}}\exp(\frac{1-2\mathrm{Re}\{\hat{q}_{nk}(i)\}}{v^{q}_{nk}(i)})}{(1+\frac{(1-\epsilon_{nk})}{\epsilon_{nk}}\exp(\frac{1-2\mathrm{Re}\{\hat{q}_{nk}(i)\}}{v^{q}_{nk}(i)}))^2}\label{eq:code_var_update}
    \end{align}
\end{subequations}

After iterating through the weak edges, we pass along the strong edges to the binary codeword variables by passing the messages
\begin{equation}
    \Delta_{c_{nk}\rightarrow f_{nk}^c}^i(c_{nk})\triangleq d^c_{nk}(c_{nk})=\mathcal{CN}(c_{nk};\hat{q}_{nk}(i),v^q_{nk}(i))
\end{equation}
Given \eqref{eq:subvector_pmf} we have $d^c_{lk}\triangleq P_{\mathbf{c}_k^{(l)}}(\mathbf{c}_k^{(l)})$ which we marginalize with respect to $c_{nk}^{(l)}$, i.e.,
\begin{multline}
    \Delta_{d^c_{kl}\rightarrow c_{nk}^{(l)}}^i(c_{nk}^{(l)})=\\
    \begin{cases}
        \Delta_{c_{nk}^{(l)}\rightarrow d_{lk}^c}^i(1)\prod\limits_{j\neq n} \Delta_{c_{jk}^{(l)}\rightarrow d_{lk}^c}^i(0)&c_{nk}^{(l)}=1\\
        \frac{1}{Q}\sum\limits_{j\neq n}\Delta_{c_{jk}^{(l)}\rightarrow d_{lk}^c}^i(1) \prod\limits_{v\neq j} \Delta_{c_{uk}\rightarrow d_{lk}^c}^i(0)&c_{nk}^{(l)}=0
    \end{cases}
\end{multline}

from which we compute the belief updates for the binary vector elements by marginalizing over $d_{lk}^c$ which results in following messages
\begin{equation}
     \Delta_{d^c_{lk}\rightarrow c_{nk}^{(l)}}^{i+1}(c_{nk}^{(l)}=1)\triangleq \hat{\epsilon}_{nk}^{(l)}(i+1)\triangleq \hat{\epsilon}_{nk}^{i+1}=    \left(1+Q\sum_n \exp(\frac{1-2\mathrm{Re}\{\hat{q}^{(l)}_{nk}(i)\}}{v^{q,(l)}_{nk}(i)})\right)^{-1}.
\end{equation}

\begin{multline}
\Delta_{d^c_{lk}\rightarrow c_{nk}^{(l)}}^{i+1}(c_{nk}^{(l)}=1)\triangleq\\
\left(1+Q\sum_n \exp(\frac{1-2\mathrm{Re}\{\hat{q}^{(l)}_{nk}(i)\}}{v^{q,(l)}_{nk}(i)})\right)^{-1}.
\end{multline}
The beliefs $\hat{\epsilon}_{nk}^{i+1}$ are passed as extrinsic information to the outer \ac{SISO} channel for single user decoding.

% \subsubsection{Message Updates of Strong Edges}
% After iterating through the weak edges, we pass along the strong edges to the binary codeword variables by passing the messages
% \begin{equation}
%     \Delta_{s_{nk}\rightarrow f_{nk}^s}^i(s_{nk})\triangleq d^s_{nk}(s_{nk})=\mathcal{CN}(s_{nk};\hat{q}_{nk}(i),v^q_{nk}(i))
% \end{equation}
% Given \eqref{eq:subvector_pmf} we have $d^s_{lk}\triangleq P_{\mathbf{s}_k^{(l)}\vert \lambda_k}(\mathbf{s}_k^{(l)}\vert\lambda_k)$ which we marginalize with respect to $\mathbf{s}_k^{(l)}$ to get the subsequent messages to the activity variable $\lambda_k$
% \begin{equation}
%     \Delta_{d^s_{kl}\rightarrow \lambda_k}^i(\lambda_k)=\begin{cases}
%         \frac{1}{M}\sum\limits_n \Delta_{s_{nk}^{(l)}\rightarrow d_{lk}^s}^i(1)\prod\limits_{j\neq n} \Delta_{s_{jk}^{(l)}\rightarrow d_{lk}^s}^i(0)&\lambda_k=1\\
%         \prod\limits_n \Delta_{s_{nk}\rightarrow d_{lk}^s}^i(0)&\lambda_k=0
%     \end{cases}
% \end{equation}
% which we represent for convenience in log-likelihood ratio form
% \begin{equation}
%     \mathrm{LLR}_{d^s_{lk}\rightarrow \lambda_k}^i=\log \sum_n \exp(\frac{2\hat{q}_{nk}^{(l)}(i)-1}{v^{q,(l)}_{nk}(i)}) -\log M.
% \end{equation}
% For the message from the channel side we have
% \begin{equation}
% \Delta_{d^h_{km}\rightarrow \lambda_k}^i(\lambda_k)=\lambda_k\mathcal{CN}(0;\hat{r}_{km}(i),v^k_{km}(i)+1)+(1-\lambda_k)\mathcal{CN}(0;\hat{r}_{km}(i),v^k_{km}(i))
% \end{equation}
% conveniently written as log-likelihood ratios
% \begin{equation}
%     \mathrm{LLR}_{d^h_{km}\rightarrow \lambda_k}^i=\log\frac{v^k_{km}(i)}{v^k_{km}(i)+1}+\frac{\vert \hat{r}_{km}(i)\vert^2}{v^k_{km}(i)(v^k_{km}(i)+1)}
% \end{equation}
% The user activity belief update for the next iteration can now be given by
% \begin{equation}
% \mathrm{LLR}_{\lambda_k}^{i+1}=\log \rho_k/(1-\rho_k)+\sum_l \mathrm{LLR}_{h^s_{kl}\rightarrow \lambda_k}^i + \sum_m \mathrm{LLR}_{d^h_{km}\rightarrow \lambda_k}^i
% \end{equation}
% from which the probability of activation can be derived as
% \begin{equation}
%     \hat{\rho}_k^{i+1}\triangleq (1+\exp -\mathrm{LLR}_{\lambda_k}^{i+1})^{-1}
% \end{equation}
% After passing the belief updates for the user activity $\hat{\rho}_k^{i+1}$ we compute the belief updates for the binary vector elements by marginalizing over $d_{lk}^s$ which results in following messages
% \begin{equation}
%      \Delta_{d^s_{lk}\rightarrow s_{nk}^{(l)}}^{i+1}(s_{nk}^{(l)}=1)\triangleq \hat{\epsilon}_{nk}^{(l)}(i+1)\triangleq \hat{\epsilon}_{nk}^{i+1}=     \left(1+M\frac{(1-\hat{\rho}_k^{i+1})}{\hat{\rho}_k^{i+1}}\sum_n \exp(\frac{1-2\hat{q}_{nk}^{(l)}(i)}{v^{q,(l)}_{nk}(i)})\right)^{-1}
% \end{equation}
% After computing the updated beliefs $\hat{\epsilon}_{nk}^{i+1}$ and $\hat{\rho}_{k}^{i+1}$, the belief are passed as prior to the weak edge factor graph in the subsequent turbo iteration. This procedure is repeated until some convergence criterion is met.
